# Supplementary material for: Unsupervised Domain Adaptation of a Pretrained Cross-Lingual Language Model
Source: arXiv:2011.11499 source file (2020-11-23)
Supplement: Supplementary file 1 [file appendix.tex]

\section{Experimental Details}
Here we provide the architectural details and settings for our experiments, including datasets formulation, unsupervised feature decomposition module, and task-specific module.

\subsection{Datasets Formulation}
In this paper, we consider a setting where we only have labeled data $D_{s,s}=\{(x_i^{s,s}, y_i^{s,s})|_{i=1}^{n_{s,s}}\}$ from a specific language and a specific domain which we call source language and source domain, and we want to train a classifier to be tested on data $D_{t,t}=\{(x_i^{t,t}, y_i^{t,t})|_{i=1}^{n_{t,t}}\}$ from a different language and a different domain which we call target language and target domain. We also assume access to some unlabeled data $D_{s,t}=\{(x_i^{s,t})|_{i=1}^{n_{s,t}}\}$ from the source language and the target domain, which is usually feasible in practical applications. We call this setting unsupervised cross-lingual and cross domain (CLCD) adaptation. 
In short, $D_{s,s}$ is introduced for training the task-specific module, while  $D_{s,t}$ is used for training the unsupervised feature decomposition module.
$D_{t,t}$ is presented for evaluating the performance of the whole model, i.e., the combination of the two modules.

% As illustrated in Figure~\ref{fig:mcl,}, the proposed method consists of three components: 
% a pretrained multilingual embedding module which embeds the input document into a language irrelevant representation, an unsupervised feature decomposition (UFD) module which extracts domain-invariant features and domain-specific features from the entangled language-irrelevant representation, and a task-specific module trained on the extracted domain-invariant features. We adopt XLM~\cite{lample2019cross} as the multilingual embedding module in our method, which has been pre-trained by large-scale parallel and monolingual data from various languages and is the current state-of-the-art cross-lingual language model. We describe the other two components and the training process in following subsections.

\subsection{Unsupervised Feature Decomposition}
The proposed unsupervised feature decomposition module is built upon the pretrained XLM-R cross-lingual language model and comprises of a domain-invariant feature extractor $\mathcal{F}_s$, a domain-specific feature extractor $\mathcal{F}_p$, and mutual information discriminator $T$.
% Before elaborating on our proposed unsupervised domain adaptation module, we first present some preliminary knowledge about mutual information estimation in unsupervised representation learning, which is necessary to intuitively comprehend the unsupervised domain adaptation process.
% Mutual Information Neural Estimation (MINE) \cite{belghazi2018mutual} learns to estimate the mutual information (MI) of two continuous variables $X$ and $Y$ by training a classifier to distinguish samples from the joint of $X$ and $Y$, $\mathbb J$, and the product of marginals of $X$ and $Y$, $\mathbb M$.
% MINE utilizes a lower-bound of MI based on the Donsker-Varadhan representation (DV) of the KL-divergence \cite{donsker1983asymptotic},
% \begin{equation}
%   \begin{aligned}
%     \mathcal{I}(X;Y):= \mathcal{D}_{KL}(\mathbb{J}||\mathbb{M}) \geq \widehat{\mathcal{I}}^{DV}(X;Y)\\
%     :=E_\mathbb{J}[T_\omega(x,y)]-\log E_\mathbb{M}[e^{T_\omega(x,y)}]
%   \end{aligned}
% \end{equation}
% where $T_\omega : X \times Y \mapsto \mathbb{R}$ is a discrimination function parameterized by a neural network with learnable parameters $\omega$. 
% In applications, most scenarios merely demand to maximize or minimize the estimation of MI rather than its precise value.

\subsubsection{Domain-Invariant Feature Extractor}
We first utilize the XLM-R model to encode each document $x_i^{s,t}$ from $D_{s,t}$ into a sequence of vectors which refer to the hidden states of the XLM-R last layer. 
We then treat the average of each sequence of vectors as the representation of each document, denoted as $h_i^{s,t}$. The dimension of the XLM-R hidden states is 1024, i.e., $h_i^{s,t}$ $\in R^{1024}$.
The domain-invariant feature extractor $\mathcal{F}_s$ consists of two feed-forward layers. 
The first layer takes the vector presentation of each document $h_i^{s,t}$ as input and output a 1024-dimension intermediate representation, formulated as
\begin{equation}
  \begin{aligned}
    v_{i,s}^{s,t} = relu(W_1h_i^{s,t} + b_1)\\
    v_{i,s}^{s,t} = v_{i,s}^{s,t} + h_i^{s,t} 
  \end{aligned}
\end{equation}
where $W_1$ $\in R^{1024 \times 1024}$ and $b_1$ $\in R^{1024}$ are trainable parameters of the first layer, and the addition operation between the input and the output of the first layer refers to the residual connection. 
Similarly, the second feed-forward layer takes $v_{i,s}^{s,t}$ as input and output the domain-invariant feature $f_{i,s}^{s,t}$ with dimension of 1024, written by
\begin{equation}
  \begin{aligned}
    f_{i,s}^{s,t} = relu(W_2v_{i,s}^{s,t} + b_2)\\
    f_{i,s}^{s,t} = f_{i,s}^{s,t} + v_{i,s}^{s,t} 
  \end{aligned}
\end{equation}
where $W_2$ $\in R^{1024 \times 1024}$ and $b_2$ $\in R^{1024}$ are trainable parameters of the second layer.

\subsubsection{Domain-Specific Feature Extractor}
The domain-specific feature extractor $\mathcal{F}_p$ takes the vector presentation of each document $h_i^{s,t}$ as input and output the corresponded intermediate representation $v_{i,p}^{s,t}$ by
\begin{equation}
  \begin{aligned}
    v_{i,p}^{s,t} = relu(W_3h_i^{s,t} + b_3)
  \end{aligned}
\end{equation}
where $W_3$ $\in R^{1024 \times 1024}$ and $b_3$ $\in R^{1024}$ are trainable parameters of the first layer. 
The second layer is introduced for calculating the domain-specific feature $f_{i,p}^{s,t}$ with dimension of 1024 by
\begin{equation}
  \begin{aligned}
    f_{i,p}^{s,t} = relu(W_4v_{i,p}^{s,t} + b_4)
  \end{aligned}
\end{equation}
where $W_4$ $\in R^{1024 \times 1024}$ and $b_4$ $\in R^{1024}$. 

\subsubsection{Mutual Information Discriminators}
To compute the mutual information between the input and the output of domain-invariant feature extractor $\mathcal{F}_s$, we introduce a simple one-layer mutual information discriminator $T_s$.
It takes $h_i^{s,t}$ $\in R^{1024}$ and $f_{i,s}^{s,t}$ $\in R^{1024}$ as input to output a scalar by
\begin{equation}
  \begin{aligned}
    m_{i,s}^{s,t} = relu(W_5[h_i^{s,t},f_{i,s}^{s,t}] + b_5)
  \end{aligned}
\end{equation}
where $W_4$ $\in R^{2048 \times 1024}$ and $b_4$ $\in R^{2048}$. $[\cdot]$ represents concatenation operation. 
The mutual information between $D_{s,t}$ and $\mathcal{F}_s(D_{s,t})$ is denoted as 
\begin{equation}
  \begin{aligned}
\widehat{\mathcal{I}}(D_{s,t};\mathcal{F}_s(D_{s,t})) = \sum_{i=1}^{n_{s,t}}-sp(-m_{i,s}^{s,t})-sp(m_{i^{'},s}^{s,t})
  \end{aligned}
\end{equation}
where $sp$ refers to the softplus activation function, i.e., $sp(z)=\log (1+e^z)$. $i^{'}$ is not equal to $i$, which represents randomly sampling a negative instance from the rest texts other than $x_i^{s,t}$.

To calculate the mutual information between the outputs of domain-invariant feature extractor and domain-specific feature extractor, we introduce another mutual information discriminator with the aforementioned structure but different parameters.
The corresponded mutual information is computed by  
\begin{equation}
  \begin{aligned}
\widehat{\mathcal{I}}(\mathcal{F}_p(D_{s,t});\mathcal{F}_s(D_{s,t})) = \sum_{i=1}^{n_{s,t}}-sp(-m_{i,s,p}^{s,t})-sp(m_{i^{'},s,p}^{s,t})
  \end{aligned}
\end{equation}

\subsubsection{Training}
The objective of the unsupervised feature decomposition (UFD) module is to maximize the mutual information $\widehat{\mathcal{I}}(D_{s,t};\mathcal{F}_s(D_{s,t}))$ and meanwhile minimize the mutual information $\widehat{\mathcal{I}}(\mathcal{F}_p(D_{s,t});\mathcal{F}_s(D_{s,t}))$. Thus, the loss value of mutual information maximization $\mathcal{L}_{s}$ refers to -$\widehat{\mathcal{I}}(D_{s,t};\mathcal{F}_s(D_{s,t}))$ and the loss value of mutual information minimization $\mathcal{L}_{p}$ is $\widehat{\mathcal{I}}(\mathcal{F}_p(D_{s,t});\mathcal{F}_s(D_{s,t}))$.
Besides, we also introduce another loss signal to minimize the mutual information between the intermediate representations of $\mathcal{F}_s$ and $\mathcal{F}_p$, denoted as $\mathcal{L}_{m}$, where the mutual information is calculated by the mutual information discriminator of $\mathcal{L}_{p}$. 
We utilize balancing parameters to combine three different losses
\begin{equation}
  \begin{aligned}
\mathcal{L}_{UFD} = \alpha\mathcal{L}_s + \beta\mathcal{L}_m + \gamma\mathcal{L}_p
  \end{aligned}
\end{equation}
where $\alpha, \beta, \gamma$ are set to 1, 0.2, 1, respectively.
The final objective of the unsupervised feature decomposition module is to minimize $\mathcal{L}_{UFD}$.

\subsection{Task-Specific Module}
To reduce the demand for labeled texts, the task-specific module is parameterized as a simple one-layer fully connected network with the softmax function to output the task label, which is also recommended in combining pretrained language models with downstream tasks. 
The input of the task module are the domain-invariant feature representation $f_{i,s}^{s,s}$ of an input text from the source language and source domain $x_i^{s,s}$ and the correlated domain-specific feature representation $f_{i,p}^{s,s}$.
The output of the task-specific module is obtained by
\begin{equation}
  \begin{aligned}
    y_i^{s,s'} = softmax(W_6[f_{i,s}^{s,s},f_{i,p}^{s,s}] + b_6)
  \end{aligned}
\end{equation}
where $W_4$ $\in R^{2048 \times 1024}$ and $b_4$ $\in R^{2048}$. 
We then utilize cross-entropy to calculate the task-specific loss.

\begin{table*}[t]
\begin{center}
\footnotesize
\resizebox{\textwidth}{!}{
\begin{tabular}{|l|l||c c c c||c c c c|| c c c c |}
\hline
\multirow{2}*{} &\multirow{2}*{\bf Settings } & \multicolumn{4}{c||}{\bf German} & \multicolumn{4}{c||}{\bf French} & \multicolumn{4}{c|}{\bf Japanese}\\
\cline{3-14}
& & \bf~Books~ & \bf ~DVD~ &\bf ~Music~ & \bf ~Avg~ & \bf~Books~ & \bf ~DVD~ &\bf ~Music~ & \bf ~Avg~ & \bf~Books~ & \bf ~DVD~ &\bf ~Music~ & \bf ~Avg~\\
\hline
\hline
\multirow{8}*{Domain-Invariant}& Max-10 & 82.4&	79.9&	78.9&	80.4& 	78.9&	80.4&	81.0&	80.1&	78.2&	79.2&	76.6&	78.0\\
&Max-50 & 76.5&	79.6&	74.5& 76.9&		77.5&	79.5&	76.0&	77.7&	79.9&	78.9&	79.0&	79.2\\
& Max-Min-10 & 76.5&	80.5&	81.7&	79.6&		70.7&	79.7& 79.8&	76.7&	78.1&	78.7&	82.3&	79.7\\
&Max-Min-50 &84.5&	78.9&	80.5&	81.3&		82.4&	80.8&	81.3&	81.5&	76.7&	79.5&	79.2&	78.4\\
&2Max-Min-10 & 83.4&	75.8&	81.5&	80.2&	80.3& 79.3&	82.3&	80.6&	77.4&	77.5&	81.8&	78.9\\
&2Max-Min-50 & 90.3&	80.4&	81.3&	84.0&	90.3&	80.9&	84.2&	85.1&	81.3&	78.0&	80.2&	79.8\\
&2Max-2Min-10&82.5&	75.1&	78.6&	78.7&		79.4&	78.4&	79.1&	79.0&	77.5&	77.9&	78.3&	77.9\\
&2Max-2Min-50&81.4&	77.9&	81.0&	80.1&	78.7&	79.1&	82.9&	80.2&	80.3&	78.7&	79.6&	79.5\\
\hline
\multirow{8}*{Invariant-Specific} & Max-Min-10 & 87.4&	83.4&	88.7&	86.5&	88.4&	89.1&	89.2&	88.9&	83.5&	83.1&	83.4& 83.3\\
& Max-Min-50 & 87.0&	87.4&	88.7&	87.7& 89.1&	89.1&	88.0&	88.7& 83.9&	84.1&	84.&	84.3\\
& Max-2Min-10 &89.2&	85.3&	88.0&	87.5&	89.2&	86.6&	85.4&	87.0&	83.5&	80.3&	84.8&	82.9\\
& Max-2Min-50 & 84.3&	86.6&	86.9&	85.9&		89.1&	88.5&	89.2&	88.9&	82.1&	85.9&	85.3& 84.4\\
& 2Max-Min-10 &90.2& 83.9&	75.5&	83.2&	88.2&	87.9&	86.5&	87.5&	83.8&	83.9&	84.8&	84.1\\
& 2Max-Min-50 & 89.1&	86.1&	87.1&	87.4&	88.3&	88.2&	86.6&	87.7& 84.0&	85.6&	81.8&	83.8\\
& 2Max-2Min-10 &88.5&	85.6&	87.5&	87.2&	86.9&	88.6&	88.6&	88.0&	83.7& 83.9&	83.7&	83.8\\
& 2Max-2Min-50 & 89.0&	86.6&	87.7&	87.8&		89.4&	87.7&	88.6&	88.5&	83.3&	83.5&	84.4&	83.7\\
\hline
\hline
\multirow{5}*{Model Ablation}& Max &83.7&	83.1&	80.3&	82.3&	82.9&	84.0&	82.1&	83.0&	81.5&	80.8&	81.3&	81.2\\
&Max-Min &89.2&	86.2&	88.1&	87.8&	87.7&	88.2&	87.5&	87.8&		83.9&	82.9&	84.6&	83.8\\
&Max-2Min & 88.6&	85.8&	87.7&	87.3&	88.4&	87.6&	88.8&	88.3& 82.5&	83.4&	83.7&	83.2\\
&2Max-Min & 89.2&86.4&	88.8&\bf	88.1&		89.5&	89.4&	89.1&	\bf89.3&	83.8&	84.5&	85.2&\bf	84.5\\
&2Max-2Min &89.6&	86.4&	87.7&	87.9&		89.1&	88.5&	88.6&	88.7&	83.4&83.8&	84.8&	84.0\\
% & MAN-MOE &82.4 & 78.8 & 77.2 &79.5  &81.1 &  84.3 & 80.9 &82.1& 62.8  &69.1 & 72.6 &68.2\\
\hline
\end{tabular}}
\caption{\label{tab:appendix_ablation}Domain-Invariant refers to only utilizing domain-invariant features for the sentiment classification task, where "-10" and "-50" refer to utilizing 10K and 50K source language target domain raw data; Invariant-Specific represents using both domain-invariant and domain-specific features for classification; Model ablation refers to the experimental results of different combinations of model components. In this setting, we utilize 50K*3 raw text from three different domains in the source language. }
% \vspace{-0.3cm}
\end{center}
\end{table*}

\begin{table*}[t]
\begin{center}
\footnotesize
\resizebox{\textwidth}{!}{
\begin{tabular}{|l|l||c c c c||c c c c|| c c c c |}
\hline
\multirow{2}*{} &\multirow{2}*{\bf Settings } & \multicolumn{4}{c||}{\bf German} & \multicolumn{4}{c||}{\bf French} & \multicolumn{4}{c|}{\bf Japanese}\\
\cline{3-14}
& & \bf~Books~ & \bf ~DVD~ &\bf ~Music~ & \bf ~Avg~ & \bf~Books~ & \bf ~DVD~ &\bf ~Music~ & \bf ~Avg~ & \bf~Books~ & \bf ~DVD~ &\bf ~Music~ & \bf ~Avg~\\
\hline
\hline
\multirow{4}*{Max-2Min} &50K*3-run1 & 89.1& 86.1&88.8&	88.0&		89.8&	89.1&	88.7&	89.2&		80.4&	82.6&	82.0&	81.7\\
&50K*3-run2 & 89.2&	86.2&	87.5&	87.6&	89.8&	88.1&	88.7&	88.9&		84.8&	84.6&	85.6&	85.0\\
&50K*3-run3& 87.5&	85.1&	86.8&	86.5&	85.6&	85.6&	89.1&	86.8&		82.3&	83.1&	83.6&	83.0\\
&50K*3-Average& 88.6&	85.8&	87.7&	87.3&	88.4&	87.6&	88.8&	88.3& 82.5&	83.4&	83.7&	83.2\\
\hline
\multirow{8}*{2Max-Min}& 1K*3 &90.2&	86.6&	87.7&\bf	88.1&		89.7&	88.6&	87.4&	88.6&	77.2&	76.6&	81.8&	78.5\\
&2K*3& 89.1&	86.9&	86.7&	87.6&		86.6&	86.9&	75.6&	83.0&	85.1&	85.1&	85.7&	85.3\\
&5K*3& 88.7&	86.4&	88.2&	87.8&	86.9&	88.5&	84.8&	86.7&	80.6&	83.2&	84.8&	82.9\\
&10K*3 & 89.0&	86.6&	88.6&\bf	88.1&		88.8&	88.2&	87.4&	88.1&		84.1&	86.2&	85.9&\bf	85.4\\
&50K*3-run1 & 90.5&	86.6&	89.3&	88.8&		89.6&	89.5&	89.7&	89.6&	84.3&	84.8&	86.8&	85.3\\
&50K*3-run2 & 88.8&	86.3&	88.9&	88.0&	89.7&	89.4&	88.5&	89.2&		83.6&	83.8&	85.3&	84.2\\
&50K*3-run3& 88.4&	86.2&	88.3&	87.6&		89.1&	89.3&	89.0&	89.1&	83.4&	84.9&	83.5&	83.9\\
&50K*3-Average& 89.2&86.4&	88.8&\bf	88.1&		89.5&	89.4&	89.1&\bf	89.3&	83.8&	84.5&	85.2&	84.5\\
\hline
\multirow{8}*{2Max-2Min} & 1K*3 & 88.6&	86.5&	87.7&	87.6&	88.9&	88.7&	87.5&	88.3&	84.7&	84.4&	85.1&	84.7\\
&2K*3& 85.4&	84.9&	85.3&	85.2&		86.9&	87.1&	86.1&	86.7&		84.8&	85.3&	85.3&\bf	85.1\\
&5K*3& 88.2&	86.7&	88.0&	87.6&		89.6&	89.4&	88.1&	89.0&		84.3&	85.3&	83.5&	84.3\\
&10K*3 & 90.3&	86.8&	87.2&\bf	88.1&		90.4&	88.9&	89.8&	\bf 89.7&	84.7&	83.8&	82.0&	83.5\\
&50K*3-run1 & 90.3&	87.1&	88.6&	88.7&		89.5&	90.0&	89.5&	89.7&	83.0&	83.5&	84.8&	83.8\\
&50K*3-run2 & 89.4&	86.1&	88.2&	87.9&	88.1&	86.7&	87.5&	87.4&		84.2&	83.0&	85.4&	84.2\\
&50K*3-run3& 89.0& 86.0&	86.5&	87.2&	89.8&	88.8&	88.8&	89.1&		83.2&	84.9&	84.3&	84.1\\
&50K*3-Average& 89.6&	86.4&	87.7&	87.9&		89.1&	88.5&	88.6&	88.7&	83.4&83.8&	84.8&	84.0\\
\hline
\end{tabular}}
\caption{\label{tab:appendix_size} Classification accuracy of using different sizes of unlabeled raw data in the source language (i.e. English).}
\end{center}
\end{table*}
